# Supplementary material for: USB Gym: A Gymnasium Testbed for Closed-Loop Ultrasound View Matching
Source: arXiv:2611.08352 source file (2026-12-03)
Supplement: Supplementary file 1 [file supp_labels.tex]

\makeatletter
\newlabel{fig:stages}{{A.1}{4}{What the testbed renders: one held-out view under the four reference texture stages, from patient s0513 at the target pose of its first screened liver window (top) and kidney window (bottom). Left: the CT label map, with orange liver, green gallbladder, blue vessel, pink kidney and gray other tissue. Physics: the sector-warped render without domain randomization and with a fixed speckle seed, in which liver and surrounding tissue are nearly isoechoic (Section~\ref {sec:rendering}). CUT, CycleGAN and SonoSPADE act on that frame, and SonoSPADE also receives the label map. Supplementary Fig.~S3.1 shows the same patient under the renderer-slot simulators. The figure is qualitative.\relax }{figure.caption.2}{supplementary.pdf}}
\newlabel{app:eval}{{Supplementary Appendix\nobreakspace  {}A}{4}{Evaluation details and supporting results}{appendix.supp.app.A}{supplementary.pdf}}
\newlabel{app:scene}{{Supplementary Appendix\nobreakspace  {}A.1}{4}{Case split and reference texture stages}{subsection.supp.app.A.1}{supplementary.pdf}}
\newlabel{app:checks}{{Supplementary Appendix\nobreakspace  {}A.2}{4}{Details of the controls}{subsection.supp.app.A.2}{supplementary.pdf}}
\newlabel{tab:posthoc-keepbest}{{A.1}{7}{Keep-best error against final error, contact on (post hoc). Keep-best is the translation error at the step of highest match score $S$, a selection that reads no pose. The 12-step rows are the episodes of Table~\ref {tab:ladder}, seeds pooled; four-stage rows average the four stages. The 36-step rows are exploratory. Plug rows use the episodes and seeds of Table~\ref {tab:pluggability}. $^{\dagger }$Privileged.\relax }{table.caption.11}{supplementary.pdf}}
\newlabel{fig:ladder}{{A.2}{8}{Mean translation error against control step on the six held-out patients, with contact on and no domain randomization at evaluation (post hoc). Lines show the static start, the pose oracle, the CT-mask servo base and final policies, and the learned-mask final policies. The CT-mask servos improve up to step 12, while three learned-mask policies are lowest at step 4 or 5 and then drift away. Supplementary Fig.~S2.1 shows each patient's final error on every rung. Every contrast is conditional on the trained artifacts (texture networks, segmenters, bases and policies). Seeds index artifacts; the patient is the sampling unit.\relax }{figure.caption.13}{supplementary.pdf}}
\newlabel{app:learnability}{{Supplementary Appendix\nobreakspace  {}A.3}{8}{Appearance-term learnability}{subsection.supp.app.A.3}{supplementary.pdf}}
\newlabel{tab:learnability}{{A.2}{9}{Appearance-term learnability on the 6 held-out patients. Each target view (5 per patient and organ, 60 in all) is compared with 40 nearby probe poses; the per-view score is the Spearman correlation between the sector-interior appearance match and closeness to the target pose. (a) SonoSPADE against each other stage: mean per-view Spearman of both stages, the mean over patients of the per-patient difference in mean Fisher-$z$ ($\Delta z$), its 95\% patient-cluster bootstrap CI, and the number of patients that share its sign. Rule: a difference under the CI-and-sign rule. The pooled rows are the pre-specified primary contrast. (b) Exploratory renderer-term ablation, not pre-specified: mean per-view Spearman with one renderer term switched off. Interface reflection off: no transmission loss or specular echo at tissue interfaces, attenuation kept. Diffuse scattering off: scattering strength 0. Depth variation of the PSF off: a depth-invariant lateral width. Flat means the appearance term is constant over poses, so the correlation is undefined. DR is off throughout.\relax }{table.caption.16}{supplementary.pdf}}
\newlabel{app:dr}{{Supplementary Appendix\nobreakspace  {}A.4}{9}{DR knobs and the DR landscape}{subsection.supp.app.A.4}{supplementary.pdf}}
\newlabel{tab:dr}{{A.3}{10}{Domain-randomization (DR) knobs. When DR is on, each knob is drawn uniformly from its range once per episode and shared by the target and the observations. DR is off in training and evaluation for Tables~\ref {tab:ladder} and~\ref {tab:learnability}; Table~\ref {tab:contact-dr} reports the DR arms. Effect: mean absolute change of the in-sector pixel intensity (scale 0 to 1, $\times 100$) when the knob alone moves to the low (lo) or high (hi) end of its range, with the speckle seed fixed, over 60 frames (6 held-out patients $\times $ 10 jittered window poses), with each texture stage applied (physics: none). $^{\dagger }$Drawn independently per tissue label and measured one label at a time (mean over labels covering at least 1\% of the sector). The speckle and noise seed is also redrawn per episode. The reference rows give the change from a new seed alone, a 5~mm in-plane slide and a full DR draw (5 draws per frame, 300 in all). The two weakest knobs, impedance multiplier and overall gain, change the frame by at most 0.21 and 0.48.\relax }{table.caption.17}{supplementary.pdf}}
\newlabel{app:contact-dr}{{Supplementary Appendix\nobreakspace  {}A.5}{10}{Contact and DR in the closed loop}{subsection.supp.app.A.5}{supplementary.pdf}}
\newlabel{tab:contact-dr}{{A.4}{11}{Contact and domain-randomization (DR) contrasts on the final pose error (mm), 6 held-out patients, 3 seeds, the crossed episodes of Table~\ref {tab:ladder}. Contact rows: contact switched off at evaluation only, minus contact on, for every rung. The static start never moves, so its delta is 0 to numerical precision. The reference rungs and the CT-mask servo base do not depend on the texture stage and give one value (all). DR rows: the SonoSPADE CT-mask arm with DR in evaluation, in training, or in both, minus the same arm without DR (11.69~mm); these rows are descriptive. Each row gives the mean of per-patient paired differences, a 95\% patient-cluster bootstrap CI and the number of patients that share the sign of the mean. $^{\ast }$: a difference under the CI-and-sign rule. $^{\mathrm {H}}$: also passes Holm on the paired $t$-test over the 16 contact rows (post hoc; Supplementary Table~S2.18); 5 of the 14 starred rows do not.\relax }{table.caption.18}{supplementary.pdf}}
\newlabel{app:identity}{{Supplementary Appendix\nobreakspace  {}A.6}{11}{Distance to real frames and organ identity}{subsection.supp.app.A.6}{supplementary.pdf}}
\newlabel{tab:posthoc-axes}{{A.5}{12}{Per-axis final error with contact on and off, 12 steps, the 60 held-out episodes (post hoc). Errors are patient-level means of the absolute SE(3)-log component in the target probe frame: lateral, elevational and axial translation, and out-of-plane tilt, in-plane tilt and roll. Base and policy rows pool seeds 0 to 2; four-stage rows also pool the four texture stages. In contact is the share of steps in contact. Gap is the mean height of the lowest face point above the plane, negative when pressed in. Lag is the mean distance between commanded and actual probe position after a step. The episodes are those of Table~\ref {tab:ladder}. $^{\dagger }$Privileged.\relax }{table.caption.19}{supplementary.pdf}}
\newlabel{app:registration}{{Supplementary Appendix\nobreakspace  {}A.7}{12}{Offline registration and matched layout}{subsection.supp.app.A.7}{supplementary.pdf}}
\newlabel{fig:layout}{{A.3}{13}{Simulated and real frames in matched sector geometry. Each row pairs one annotated public real frame from the Vitale test set \cite {vitaledata,vitale} with the held-out CT view whose organ layout best matches its annotation; the row label gives the frame, the CT patient and the organ-layout IoU of the match. For each real frame, the search scored 2,000 candidate probe poses per held-out patient around the screened acoustic windows by mean per-organ IoU and refined the best three by a cross-entropy search; a pose rotated by 180 degrees about the beam axis was also allowed. The search used label maps only, and no rendered image entered it. The columns show the real frame with its annotation outlined, the annotation, the matched CT label, and the physics, CUT, CycleGAN and SonoSPADE renders at the matched pose (no domain randomization, fixed speckle seed) with the CT label outlined (orange liver, green gallbladder, blue vessel, pink kidney, yellow spleen). The rows follow a fixed rule: the best frame of each organ stratum that has at least three frames, then the global IoU rank, with at most two rows per patient. Over all 60 frames, the median best IoU is 0.56 (interquartile range 0.42 to 0.81). \relax }{figure.caption.23}{supplementary.pdf}}
\newlabel{tab:realism}{{A.6}{14}{Distance to real B-mode frames in matched sector geometry. Simulated side: 50 views per held-out patient (6 patients, 300 views) jittered around screened acoustic windows, warped to the real sector. Real side: the 60 annotated Vitale frames~\cite {vitale}, which no texture stage trained on. All scores use in-sector pixels only (sector mask eroded by 3~px). W1: intensity Wasserstein-1 distance. KID and FID: kernel and Fr\'echet Inception distances. C2ST AUC: area under the ROC curve of a CNN classifier two-sample test, mean $\pm $ std over 5 repeats $\times $ 5 grouped folds (0.5 means the classifier cannot separate the domains). KID: mean $\pm $ std over 100 random subsets of 50 frames per domain. Lower W1, KID and FID mean a smaller distance to the real frames. FID from 60 real frames is biased upward and is printed for completeness; KID is the unbiased kernel distance. NumPy renderer: the five-tissue appearance model of the authors' earlier simulator (Supplementary Table~S1.3). A post hoc label-permutation null with 200 permutations per stage gives a mean AUC of 0.50 (SD 0.07) for every stage and never reaches the observed AUC of any stage ($p = 1/201$ each). Physics W1 is below the authors' reimplementation of LOTUS in 6/6 held-out patients and is below it pooled. In a post hoc comparison with the original LOTUS code, physics W1 is lower in 5/6 patients and lower pooled. Supplementary Table~S2.16 gives the null per stage and post hoc frame-bootstrap intervals for W1 and KID. The established-simulator rows run the same protocol with the renderer swapped (exploratory). The original LOTUS code runs with its published default parameters.\relax }{table.caption.20}{supplementary.pdf}}
\newlabel{app:posthoc-best}{{Supplementary Appendix\nobreakspace  {}A.8}{14}{Post hoc lowest-error pipelines}{subsection.supp.app.A.8}{supplementary.pdf}}
\newlabel{tab:identity}{{A.7}{15}{Cross-domain organ identity of each stage's texture-matched segmenter. A cell counts the segmenter seeds, of 3, on which the modal predicted class of the organ is the correct class both in simulation (288 frames from the held-out patients) and on real frames. Liver, gallbladder (GB), vessel and spleen are scored on Vitale~\cite {vitale}: all 60 annotated frames, each predicted by a model that never trained on it (top), or only the 18 holdout frames that no segmenter trained on (bottom). Kidney is scored on the KidneyUS holdout~\cite {kidneyus} (107 frames) in both panels. Last column: organs of the four (liver, GB, vessel, kidney) per seed, mean $\pm $ population std over the 3 seeds. Spleen is not a target and is descriptive only. The table is descriptive. Under the pre-specified rule, both panels detect no difference in organ-identity consistency across stages (not powered for equivalence).\relax }{table.caption.21}{supplementary.pdf}}
\newlabel{tab:registration}{{A.8}{15}{Offline registration against real target frames (no probe, phantom or robot). Each real target is paired with 3 held-out CTs. Each learned-mask servo (3 seeds) takes its masks of the real frame and of the simulated view, for control and reward, from its own segmenter. Score: organ-restricted IoU between the CT label of the simulated view and the annotated organ of the real frame, at the keep-best step (chosen by that reward, without ground truth) minus at the static start. Mean over targets (each averaged over 9 runs), with a 95\% bootstrap CI over targets. Rule met: yes only if the CI lies above 0 (pre-specified rule). AUL and KidneyUS frames are resized screenshots outside the convex-sector geometry of the renders.\relax }{table.caption.22}{supplementary.pdf}}
\newlabel{tab:real-cells-all}{{A.9}{16}{Outcomes of the eight testable real-frame cells, every texture stage of the ladder (Table~\ref {tab:real-cells} prints the rows of SonoSPADE, the standard engine's stage). Keep-best gain: primary gain over the static start (Table~\ref {tab:registration}). Selection: organ IoU of the state the match score selects along undirected motion, minus that of a random state. Directed control: the policy's keep-best gain minus that of magnitude-matched undirected motion with the same selection. Values: exploratory per-subject IoU means [95\% subject-by-CT bootstrap CI]. A cell holds if its CI excludes 0 and its Holm $p$ over eight cells is below 0.05. In the holding cell, 38/55 subjects share the sign; exact sign-flip $p = 3.4 \times 10^{-4}$ and Holm $p = 0.003$. Elsewhere Holm $p$ is 0.055 to 1.000.\relax }{table.caption.24}{supplementary.pdf}}
\newlabel{tab:best-so-far}{{A.10}{16}{Lowest measured error per kind of run-time input, post hoc. Post hoc: lowest point estimate on the same six held-out patients that measured it, so optimistic; not the pre-specified combination rule. The pre-specified combination selects by the slot decisions and tests its choice on 20 CTs that played no part in it, so the two can name different pipelines. Pipelines name the frames, the mask source and the controller. Error: final translation error over the 60 held-out episodes of Table~\ref {tab:ladder}, mean over seeds of patient means. Differences are paired by patient, with the 95\% $t$ CI and the patients of 6 sharing the sign. A random-action controller, from earlier runs with no pre-specified rule, ends at 17.45~mm (3 seeds; Supplementary Table~S3.2). Each post hoc lowest row is the lowest error among the 18, 17 and 43 measured candidates of the second, third and fourth blocks. No candidate combines the winners of two slots; the pre-specified combination is reported in Section~\ref {sec:plug-best}. The learned-mask controller arm with new learner seeds is not a candidate; its rows are in Table~\ref {tab:arm-a}. Both lowest rows without privileged input are BC residuals (exploratory, no pre-specified rule). None of these rows enters a decision, and none is read as a separation of two methods. Cohort: the same configuration on the 20-CT replication cohort, an unselected check; n/r, not run there. Every episode keeps the contact plane through the target window face and a start drawn around the target. No row is therefore free of target information. $^{\mathrm {L}}$Label-conditioned stage: its network also reads the CT label slice. $^{\dagger }$Privileged: simulator state that no rig provides. $^{\mathrm {E}}$Exploratory, no pre-specified rule.\relax }{table.caption.25}{supplementary.pdf}}
\newlabel{app:decisions}{{Supplementary Appendix\nobreakspace  {}B}{17}{Outcomes of the pre-specified comparisons and exploratory experiments}{appendix.supp.app.B}{supplementary.pdf}}
\newlabel{app:decisions-texture}{{Supplementary Appendix\nobreakspace  {}B.1}{17}{Texture stage}{subsection.supp.app.B.1}{supplementary.pdf}}
\newlabel{sec:plug-texture}{{Supplementary Appendix\nobreakspace  {}B.1}{17}{Texture stage}{section*.28}{supplementary.pdf}}
\newlabel{sec:results-texture}{{Supplementary Appendix\nobreakspace  {}B.1}{17}{Texture stage}{section*.28}{supplementary.pdf}}
\newlabel{fig:forest}{{B.1}{18}{Published methods in the plug slots, each drawn as its difference from its slot's reference component, the solid vertical line. Each line is one plugged method of the five slot families of Table~\ref {tab:pluggability}. The thin bar is the 95\% paired $t$ CI, and the thick bar is the 90\% paired $t$ CI. A filled marker means that the method is equivalent to its reference within $\pm 1$~mm, the pre-specified margin, which the dotted lines mark (post hoc, unadjusted TOST). The right column prints each difference with its 95\% CI and outcome word, and daggers mark slots under the privileged CT mask. These results are exploratory; Table~\ref {tab:pluggability} gives each slot's post hoc minimum detectable difference. Every contrast is conditional on the trained artifacts (texture networks, segmenters, bases and policies). Seeds index artifacts; the patient is the sampling unit.\relax }{figure.caption.26}{supplementary.pdf}}
\newlabel{app:decisions-mask}{{Supplementary Appendix\nobreakspace  {}B.2}{18}{Mask source}{subsection.supp.app.B.2}{supplementary.pdf}}
\newlabel{tab:pluggability-engine}{{B.1}{19}{Published methods in the three slots of the standard engine: texture stage, renderer and CT anatomy (exploratory, pre-specified rule). The engine is the physics renderer with the SonoSPADE texture stage and the reference CT labels; every slot stays pluggable. Columns, slot headers, marks and notes as in Table~\ref {tab:pluggability}; the MDD leaves out SIMUS and the painted stage.\relax }{table.caption.27}{supplementary.pdf}}
\newlabel{app:decisions-controller}{{Supplementary Appendix\nobreakspace  {}B.3}{22}{Controller}{subsection.supp.app.B.3}{supplementary.pdf}}
\newlabel{app:decisions-arma}{{Supplementary Appendix\nobreakspace  {}B.3}{23}{Learned-mask controller experiment}{section*.29}{supplementary.pdf}}
\newlabel{app:decisions-earlier}{{Supplementary Appendix\nobreakspace  {}B.3}{25}{Earlier learned-mask runs}{section*.31}{supplementary.pdf}}
\newlabel{app:decisions-reward}{{Supplementary Appendix\nobreakspace  {}B.4}{25}{Reward}{subsection.supp.app.B.4}{supplementary.pdf}}
\newlabel{tab:arm-a}{{B.2}{26}{Learned-mask controller experiment on the six held-out patients (exploratory, pre-specified rule). Families LM-D (difference) and LM-E (equivalence within $\pm 1$~mm), $m = 6$ each, Holm within each family. A difference holds if its Holm $p$ is below 0.05 and at least 5 of 6 patients share its sign (paired $t$, df 5); the exact sign-flip $p$ is printed and never decides. Absolute errors are the base's mean plus the paired difference. The servo base ends at 17.20~mm with physics frames and 13.13~mm with SonoSPADE frames, and the pose oracle at 1.53~mm. MDD from the observed SDs: 2.37 and 3.63~mm for the base contrasts, 2.69 and 4.12~mm for the learner pair, at $\alpha = 0.05$ and at Holm's first step. The separation criterion (a physics-frame difference of B1, B3 or P1 holds) is met. Crossed bootstrap: case by seed, a sensitivity check.\relax }{table.caption.30}{supplementary.pdf}}
\newlabel{app:decisions-renderer}{{Supplementary Appendix\nobreakspace  {}B.5}{27}{Renderer}{subsection.supp.app.B.5}{supplementary.pdf}}
\newlabel{sec:plug-renderer}{{Supplementary Appendix\nobreakspace  {}B.5}{27}{Renderer}{section*.32}{supplementary.pdf}}
\newlabel{app:decisions-phantoms}{{Supplementary Appendix\nobreakspace  {}B.5}{27}{Canonical phantoms}{section*.33}{supplementary.pdf}}
\newlabel{app:decisions-anatomy}{{Supplementary Appendix\nobreakspace  {}B.6}{28}{CT anatomy}{subsection.supp.app.B.6}{supplementary.pdf}}
\newlabel{sec:plug-anatomy}{{Supplementary Appendix\nobreakspace  {}B.6}{28}{CT anatomy}{section*.34}{supplementary.pdf}}
\newlabel{app:decisions-cohort}{{Supplementary Appendix\nobreakspace  {}B.7}{29}{Plugged methods on the replication cohort}{subsection.supp.app.B.7}{supplementary.pdf}}
\newlabel{app:decisions-contact}{{Supplementary Appendix\nobreakspace  {}B.8}{30}{Contact surface}{subsection.supp.app.B.8}{supplementary.pdf}}
\newlabel{tab:arm-b}{{B.3}{31}{Skin-tangent contact experiment (exploratory, pre-specified rule): skin-tangent plane minus target-anchored plane, same rung and seed, on the six held-out patients. Families SKIN-D (change) and SKIN-E (equivalence within $\pm 1$~mm), $m = 5$ each, Holm within each family; a change holds if its Holm $p$ is below 0.05 and at least 5 of 6 patients share its sign (paired $t$, df 5); the exact sign-flip $p$ is printed and never decides. Both servo bases keep the calibrations fit with the target-anchored plane. MDD from the observed SDs: 1.71~mm at $\alpha = 0.05$ and 2.51~mm at Holm's first step. Lower block: the plane quantities over the same sampled setups, per rung (n episodes: 60 setups, times 3 seeds for the bases).\relax }{table.caption.35}{supplementary.pdf}}
\newlabel{app:decisions-amos}{{Supplementary Appendix\nobreakspace  {}B.9}{32}{External cohort}{subsection.supp.app.B.9}{supplementary.pdf}}
\newlabel{tab:amos-yield}{{B.4}{35}{Yield of the AMOS external cohort (exploratory). Of 79 eligible AMOS CTs (slice spacing at most 2.5~mm), 77 passed the label check and 76 the window screen. The first 30 passes in the seeded order form the cohort. Rows: AMOS split (Tr, training; Va, validation) and native slice spacing. Windows: screened acoustic windows per CT. Every AMOS structure comes from TotalSegmentator v2 fast-mode predictions; the AMOS manual labels serve only to accept a case, which needs a liver Dice of at least 0.85 and a kidney Dice of at least 0.70, with 5~mL as the absent-kidney volume.\relax }{table.caption.36}{supplementary.pdf}}
\newlabel{tab:amos-labels}{{B.5}{35}{Agreement of the TotalSegmentator v2 labels with the AMOS manual organ labels, Dice per structure (descriptive). Accepted: the 30 cohort CTs; rejected: the 3 screened CTs rejected by the label check or the window screen. Median over the accepted CTs: liver 0.96, kidneys 0.93.\relax }{table.caption.37}{supplementary.pdf}}
\newlabel{app:decisions-combination}{{Supplementary Appendix\nobreakspace  {}B.10}{35}{Combination and benchmark baseline}{subsection.supp.app.B.10}{supplementary.pdf}}
\newlabel{tab:amos-ctanat}{{B.6}{36}{CT-anatomy context (descriptive): the five CT-anatomy rungs of the original six on TotalSegmentator labels beside the same rungs on the 30 AMOS CTs. The two columns share the label model and differ in CT source, patients, $n$, the labels of the calibration fit and the window source; they are never pooled, and no difference across them is printed. Error: final translation error, mean over seeds of case means.\relax }{table.caption.38}{supplementary.pdf}}
\newlabel{tab:amos-results}{{B.7}{36}{AMOS external cohort on 30 CTs (exploratory, pre-specified rule; external replication in simulation only). Top: the decisions. Families AMOS-P ($m = 3$) and AMOS-S ($m = 2$), two-sided Monte Carlo sign-flip test (1,000,000 sign vectors, seed 0), Holm within each family; the CT is the unit. C1 and C2 replicate when they hold with the sign of the original six. Middle: AMOS beside the 20 replication-cohort CTs and the original six (estimation only; no $p$, no decision; 95\% $t$ CIs). An interval that covers 0 does not show that a value is unchanged, and one that excludes 0 is not a difference that holds. Bottom: the relabeling control on the 20 cohort CTs (estimation only), the paired change and the AMOS difference side by side, never added.\relax }{table.caption.39}{supplementary.pdf}}
\newlabel{app:decisions-seed}{{Supplementary Appendix\nobreakspace  {}B.11}{40}{Patient-by-seed intervals}{subsection.supp.app.B.11}{supplementary.pdf}}
\newlabel{tab:combination}{{B.8}{41}{Combination chosen by the pre-specified rule (exploratory): the authors' original pipeline with the SSIM appearance term in the REINFORCE reward, the only slot the rule changed. Primary: the 20 replication-cohort CTs, exact sign-flip test, Holm within families CMB-D ($m = 4$, difference), CMB-E ($m = 4$, equivalence within $\pm 1$~mm, TOST) and CMB-G ($m = 2$, gap to the pose oracle, conditional on this renderer: grid-fixed speckle, no elevational beam width, rigid tissue). Each D difference compares three trained policies per arm and is conditional on those six RL runs. Other pipelines measured on these CTs print as measured and none is ranked against the combination. MDD from the observed SDs, at $\alpha = 0.05$ and at Holm's first step. The continuation prints the six held-out patients (selection-biased; estimation only), the same-procedure retraining of the match score $S$ (estimation only) and AMOS (secondary; estimation only).\relax }{table.caption.45}{supplementary.pdf}}
\newlabel{tab:patient-seed}{{B.9}{43}{Patient-by-seed intervals of the Table~\ref {tab:pluggability} rows with three seeds (exploratory). Difference and $k$/6 as in Table~\ref {tab:pluggability}. Per seed: the difference of patient means within one seed, seed $s$ of the row minus seed $s$ of the reference, for seeds 0, 1 and 2. Seeds: those whose difference shares the sign of the mean (post hoc). Patient-by-seed: the pre-specified bootstrap, which resamples patients, then seeds within each sampled patient, with the seed index paired across arms; 10,000 resamples, seed 0. Crossed: patients and seeds resampled independently, a post hoc sensitivity check with the same resamples and seed. Rows run at seed 0 only have no seed factor and are not listed. Every contrast is conditional on the trained artifacts (texture networks, segmenters, bases and policies). $^{\dagger }$Privileged.\relax }{table.caption.47}{supplementary.pdf}}
\newlabel{app:leaderboard}{{Supplementary Appendix\nobreakspace  {}C}{45}{Leaderboard of the plugged methods}{appendix.supp.app.C}{supplementary.pdf}}
\newlabel{tab:leaderboard}{{C.1}{45}{Leaderboard of the methods plugged into each slot (exploratory). Each row is the row of Table~\ref {tab:pluggability} (the guide's slots) or Table~\ref {tab:pluggability-engine} (the engine's slots) for the same method, run in its slot's condition (slot headers, as in those tables), with 12 steps, the 60 held-out episodes of Table~\ref {tab:ladder} and contact on. In each slot the reference comes first, then the rows whose difference is taken from it, by mean error, lowest first, with the privileged rows last. Rows run at seed 0 only follow the reference's seed-0 line in the same order, since their differences are taken from that line and their error is that of one seed. The order is by mean error only and is not a ranking: each row was tested against its slot's reference, not against the other rows, and where the decision is no detectable difference, the methods are not distinguished from the reference or from each other. The CT-anatomy rows keep the order of Table~\ref {tab:pluggability-engine}, since each is scored against its own reference level. Authors': our published component~\cite {usbgym}. Role: the row's group in those tables; second family: the second mask-source family or the LPIPS reward family; privileged: its group of privileged rows, which are secondary. Error, difference with its 95\% paired $t$ CI and $k$/6, and decision, with the marks L, $\dagger $, $\ddagger $, a and e, as in those tables. The pretrained-backbone differences of Table~\ref {tab:pluggability}, which have no error of their own, are left out.\relax }{table.caption.49}{supplementary.pdf}}
\newlabel{app:renderer}{{S1}{47}{Renderer specification}{appendix.supp.1}{supplementary.pdf}}
\newlabel{eq:app-fan}{{S1.1}{47}{Scan geometry and CT sampling}{equation.supp.1.1}{supplementary.pdf}}
\newlabel{tab:renderer-params}{{S1.1}{48}{Constants of the physics renderer and the sector mapping, at their defaults (DR off). DR ranges are uniform draws, made once per episode when DR is on; the three per-label multipliers are drawn independently for each label. Origin: \emph {earlier} marks a scan-geometry value carried over from the authors' earlier ultrasound simulator. \emph {LOTUS} marks a LOTUS default~\cite {velikova2023lotus}; \emph {USB Gym}, a value set in this work and not taken from LOTUS; \emph {Vitale}, a value measured on public Vitale frames~\cite {vitale}; \emph {data}, a property of the CT cases. The renderer defines no center frequency and no sound speed.\relax }{table.caption.51}{supplementary.pdf}}
\newlabel{tab:renderer-labels}{{S1.2}{49}{Acoustic values of the 13 labels and the leading-gap gel. $Z_c$ is the impedance (MRayl), and $\alpha _c$ the attenuation coefficient in the units of the LOTUS table, dB\,cm$^{-1}$\,MHz$^{-1}$, used as described in Eq.~\eqref {eq:app-E}. $b_c$ is the mean backscatter (LOTUS $\mu _0$), and $\mu _{1,c}$ and $\sigma _{0,c}$ are the scatterer density and brightness spread, which only the authors' reimplementation of LOTUS reads. Source: \emph {LOTUS}, all five values are LOTUS defaults~\cite {velikova2023lotus}, which LOTUS takes from a published liver scene and approximates for muscle, background and soft tissue; \emph {USB Gym}, set in this work and not from LOTUS. Derived columns at the defaults: backscatter relative to soft tissue, $20\log _{10}(b_c/0.45)$, and the residual round-trip slope after TGC, Eq.~\eqref {eq:app-slope}, where positive darkens what lies behind. The last column is $R$ of the step from soft tissue into the label, Eq.~\eqref {eq:app-R}.\relax }{table.caption.52}{supplementary.pdf}}
\newlabel{eq:app-maps}{{S1.2}{49}{Acoustic maps and gel coupling}{equation.supp.1.2}{supplementary.pdf}}
\newlabel{tab:renderer-compare}{{S1.3}{50}{The physics renderer against the two reference renderers of Table~\ref {tab:realism}, term by term. The first reference renderer is the authors' reimplementation of the LOTUS forward model~\cite {velikova2023lotus} with its default parameters. The NumPy renderer is the five-tissue appearance model of the authors' earlier ultrasound simulator, whose scan geometry the testbed keeps. All three render the same label slice and pass through the same resizing and sector mapping. $u$ and $\nu $ are standard normal fields, $B$ the LOTUS boundary map, $h$ a Gaussian PSF and $*$ convolution. The echo of the authors' reimplementation is $\operatorname {clip}\bigl (A\,G\,(h * s) + A\,G\,T\,r\,(h * B),\ 0,\ 1\bigr )$, with $G$ its TGC ramp and $s$ its scatterer map.\relax }{table.caption.53}{supplementary.pdf}}
\newlabel{eq:app-gel}{{S1.3}{50}{Acoustic maps and gel coupling}{equation.supp.1.3}{supplementary.pdf}}
\newlabel{eq:app-R}{{S1.4}{50}{Reflection, transmission and attenuation}{equation.supp.1.4}{supplementary.pdf}}
\newlabel{tab:renderer-cohort}{{S1.4}{51}{The 19 CT cases. Age, sex (F, M), study type and tube voltage are from the TotalSegmentator metadata, which record no contrast phase; all volumes have 1.5~mm isotropic voxels. Aorta is the median HU inside the aorta mask, an indicator of contrast. The next three columns give the share of a label's voxels, before the bone overlay, that the 300~HU rule (and no bone mask) turns into bone. GI gas is the share of GI-labeled voxels below $-200$~HU.\relax }{table.caption.54}{supplementary.pdf}}
\newlabel{eq:app-E}{{S1.5}{51}{Reflection, transmission and attenuation}{equation.supp.1.5}{supplementary.pdf}}
\newlabel{eq:app-loss}{{S1.6}{51}{Reflection, transmission and attenuation}{equation.supp.1.6}{supplementary.pdf}}
\newlabel{eq:app-env}{{S1.7}{52}{Speckle and echo formation}{equation.supp.1.7}{supplementary.pdf}}
\newlabel{eq:app-echo}{{S1.8}{52}{Speckle and echo formation}{equation.supp.1.8}{supplementary.pdf}}
\newlabel{app:renderer-psf}{{S1.6}{52}{Point spread function}{subsection.supp.1.6}{supplementary.pdf}}
\newlabel{eq:app-psf}{{S1.9}{52}{Point spread function}{equation.supp.1.9}{supplementary.pdf}}
\newlabel{app:renderer-tgc}{{S1.7}{53}{Time-gain compensation, gain and noise}{subsection.supp.1.7}{supplementary.pdf}}
\newlabel{eq:app-tgc}{{S1.10}{53}{Time-gain compensation, gain and noise}{equation.supp.1.10}{supplementary.pdf}}
\newlabel{eq:app-slope}{{S1.11}{53}{Time-gain compensation, gain and noise}{equation.supp.1.11}{supplementary.pdf}}
\newlabel{eq:app-display}{{S1.12}{53}{Log compression and display mapping}{equation.supp.1.12}{supplementary.pdf}}
\newlabel{eq:app-sector}{{S1.13}{54}{Sector mapping for view matching}{equation.supp.1.13}{supplementary.pdf}}
\newlabel{app:renderer-simus}{{S1.11}{54}{Settings of the plugged SIMUS renderer}{subsection.supp.1.11}{supplementary.pdf}}
\newlabel{app:renderer-phantoms}{{S1.13}{55}{Canonical phantoms}{subsection.supp.1.13}{supplementary.pdf}}
\newlabel{tab:phantoms}{{S1.5}{56}{Canonical digital phantoms, renderers only (descriptive; no family, no decision). Each metric: mean (SD) over the 10 speckle seeds on each renderer's native output. Bands fixed before any phantom was rendered; not scorable: a wire was not measurable in every seed. Speckle SNR: mean over SD of the amplitude, after each renderer's display map is inverted (the original LOTUS map is linear and is used as returned), in phantom H at 30 to 90~mm depth on the central 80 lines, each depth row divided by its mean, on the 512 by 160 frame before resizing and the sector warp. Rayleigh reference line of the speckle SNR, that of a Rayleigh envelope: 1.91. The band counts in the renderer headers also include design-check bands that the renderer meets by its construction; those bands are not listed. The continuation gives the wire widths and the clipped fractions.\relax }{table.caption.55}{supplementary.pdf}}
\newlabel{fig:ladder-points}{{S2.1}{58}{The oracle ladder on the six held-out patients of the article, with contact on and no domain randomization at evaluation (primary results; Table~\ref {tab:ladder} of the article gives the values). One panel per texture stage. Each point is one patient's mean final translation error, thin gray lines join a patient across rungs, and short bars mark the mean over patients. The rungs are the static start and the privileged pose oracle, then, first with CT masks and then with the stage's texture-matched segmenter, the servo base alone (hollow markers) and the servo after imitation and REINFORCE (filled markers). Blue marks the CT-mask rungs and orange the learned-mask rungs. One arrow marks the oracle-to-CT-mask gap, CT-mask final minus pose oracle, at $+10.1$ to $+10.3$~mm with 6/6 patients in every stage. The other marks the CT-to-learned-mask gap, learned-mask final minus CT-mask final, at $+4.8$ to $+5.3$~mm with physics, CUT and CycleGAN and $+1.4$~mm with SonoSPADE. Each arrow label gives the mean gap and the number of patients that share its sign. Every contrast is conditional on the trained artifacts (texture networks, segmenters, bases and policies). Seeds index artifacts; the patient is the sampling unit.\relax }{figure.caption.57}{supplementary.pdf}}
\newlabel{supp:posthoc}{{S2}{58}{Exploratory and post hoc analyses of the primary results}{appendix.supp.2}{supplementary.pdf}}
\newlabel{supp:static}{{S2.1}{58}{Post hoc comparison with the static start}{subsection.supp.2.1}{supplementary.pdf}}
\newlabel{fig:landscape}{{S2.2}{59}{Appearance-term learnability on 60 held-out target views: five liver and five kidney windows per held-out patient, 40 probe poses sampled around each target view, and no domain randomization. The appearance term is the normalized cross-correlation of the sector interior, mapped to $[0,1]$. Left: mean appearance term by translation distance to the target pose. Right: mean over views of the per-view Spearman correlation between the appearance term and closeness to the target; error bars are one standard deviation across views. The mean correlation is 0.613 for SonoSPADE and 0.542 to 0.548 for the other three stages. \relax }{figure.caption.58}{supplementary.pdf}}
\newlabel{supp:posthoc-logs}{{S2.4}{59}{Post hoc analyses of the logged trajectories}{subsection.supp.2.4}{supplementary.pdf}}
\newlabel{tab:ladder-rotation-success}{{S2.1}{60}{Post hoc, not pre-specified: rotation error, success and final match score on the crossed episodes of Table~\ref {tab:ladder}. All rows use the 6 held-out patients, contact on and evaluation DR off, with 240 episodes per reference row and 3 seeds per policy row. Rotation error: the geodesic angle between the final and target probe orientations, the norm of the SO(3) logarithm of the relative rotation. Success: the share of episodes that end within both bounds, $\leq $5~mm and $\leq $5$^{\circ }$ / $\leq $10~mm and $\leq $10$^{\circ }$. Final match score $S$: the combined score of the arm at the last step. Each cell is the mean over patients of per-patient means; rotation contrasts are in Tables~\ref {tab:imitation-base} and~\ref {tab:rl-tost}. The translation error of Table~\ref {tab:ladder} is the norm of the translational part of the SE(3) logarithm; it exceeds the probe-face displacement by at most 1.3\% at the largest logged angle.\relax }{table.caption.59}{supplementary.pdf}}
\newlabel{tab:ladder-organ}{{S2.2}{61}{Post hoc, not pre-specified: the oracle ladder of Table~\ref {tab:ladder} by target organ. Each cell gives liver / kidney: the mean over the 6 held-out patients of per-patient means over that organ's episodes (5 acoustic windows per patient and organ, 3 seeds per policy row). Contact on, evaluation DR off.\relax }{table.caption.60}{supplementary.pdf}}
\newlabel{tab:step-error}{{S2.3}{62}{Post hoc: final translation error (mm) against control step on the crossed episodes of Table~\ref {tab:ladder}, from the logged per-step trajectories. Each value is the mean over the 6 held-out patients of per-patient means, with contact on and evaluation DR off. Min: the lowest mean and its step. Improving: the share of episodes whose error fell on the last step. $S$: the mean match score at steps 0 and 12. Rotation error per step is not logged.\relax }{table.caption.61}{supplementary.pdf}}
\newlabel{tab:imitation-base}{{S2.4}{62}{Post hoc: after imitation minus the servo base alone, per configuration and texture stage (6 held-out patients, 3 seeds; contact on, evaluation DR off). Mean of per-patient paired differences, the number of patients (of 6) that share its sign, the 95\% patient-cluster bootstrap CI and the paired $t$ CI. $^{\ast }$: a difference under the CI-and-sign rule, applied here post hoc. Positive: imitation ends farther from the target than the base. The CT-mask base is the same for every stage.\relax }{table.caption.62}{supplementary.pdf}}
\newlabel{supp:posthoc-uncertainty}{{S2.5}{62}{Uncertainty of primary results}{subsection.supp.2.5}{supplementary.pdf}}
\newlabel{supp:mixed}{{S2.6}{62}{Mixed-model estimates}{subsection.supp.2.6}{supplementary.pdf}}
\newlabel{tab:stats-sensitivity}{{S2.5}{63}{Post hoc statistics sensitivity for every pre-specified ladder contrast (final translation error, mm; 6 held-out patients, 3 seeds). Mean: mean of per-patient paired differences. Bootstrap: the pre-specified 95\% patient-cluster percentile CI (10,000 resamples). $t$: 95\% CI and two-sided $p$ of the paired $t$-test (5 df). Patient $\times $ seed: 95\% crossed bootstrap CI that resamples patients and seeds independently, so seed variance enters. Exact: two-sided sign-flip $p$ over all $2^6$ sign patterns. Holm: adjusted within each family (block); over all 25 contrasts as one family, 0 survive on the exact $p$ and 4 on the $t$ $p$. Rule: the pre-specified CI-and-sign rule (yes = a difference). At $n = 6$ the smallest two-sided exact $p$ is $2/64 = 0.031$, above Holm's first threshold $0.05/m$ for every family of $m \geq 2$. No exact test on six patients therefore survives Holm in a family of two or more, and a 5/6 sign pattern has exact $p \geq 4/64$. Over 10,000 simulated null data sets of six differences, the rule declares a difference in 11.7\% (normal), 10.8\% ($t$, 3 df) and 16.3\% (skewed) of cases. Under the normal null, the $t$-test does so in 5.3\% and the exact test in 3.5\%.\relax }{table.caption.63}{supplementary.pdf}}
\newlabel{tab:rule-simulation}{{S2.6}{64}{Post hoc simulation of the pre-specified CI-and-sign rule at $n = 6$ patients: the share of 10,000 simulated data sets of six paired differences in which each procedure declares a difference (two-sided, $\alpha = 0.05$). The rule is simulated as the analysis applies it: a 95\% percentile bootstrap with the same 10,000 fixed resamples, and at least 5 of 6 patients sharing the sign of the mean. Null rows give the type-I error; $\delta $ rows give the power for normal differences with mean $\delta $ standard deviations. The exact sign-flip test assumes a symmetric null, which the skewed row violates.\relax }{table.caption.64}{supplementary.pdf}}
\newlabel{tab:rl-tost}{{S2.7}{64}{Post hoc equivalence test of the RL null on the eight trained policy configurations: REINFORCE fine-tuning at the pre-specified budget, final minus after imitation, 6 held-out patients, 3 seeds. Margin $\pm 1$~mm, the pre-specified RL threshold, applied as an equivalence margin after the results were known. TOST: two one-sided paired $t$-tests (5 df); equivalence if $p < 0.05$, that is, if the 90\% $t$ CI lies inside the margin. Sign-flip: the exact version (smallest attainable $p$ is $1/64$). Patient $\times $ seed: 90\% crossed bootstrap CI with seed variance included. Rotation: the same contrast on the final rotation error (deg), with its 95\% $t$ CI and sign consistency.\relax }{table.caption.65}{supplementary.pdf}}
\newlabel{tab:registration-crossed}{{S2.8}{65}{Post hoc reanalysis of the offline registration of Table~\ref {tab:registration}. Each real target is run with all 3 seeds and with 3 of the 6 held-out CTs (the same 3 for every seed). Keep-best gain: the pre-specified metric, keep-best minus static organ-restricted IoU. Final-step gain: final minus static IoU, with no selection. Targets: the pre-specified bootstrap over targets. Targets $\times $ seeds and targets $\times $ CTs $\times $ seeds: crossed bootstrap CIs that resample each factor independently (the latter weights the observed cells, since each target meets 3 of the 6 CTs). With 3 seeds and 6 CTs these CIs are still optimistic. Holm: target-level paired $t$-test $p$, Holm-adjusted over the 16 cells. Subjects are not logged, so targets are resampled by frame, not clustered by subject. IoU: static / final / keep-best.\relax }{table.caption.66}{supplementary.pdf}}
\newlabel{tab:seg-sim-real}{{S2.9}{65}{Post hoc: Dice of each stage's texture-matched segmenter on held-out simulated frames (renders of the 6 evaluation CTs, never seen in training, each with its own domain-randomization draw, not the default evaluation render) and on real holdout frames, seeds 0 / 1 / 2. Vitale-holdout and KidneyUS frames come from datasets whose training splits the segmenters saw; AUL frames come from a dataset that no segmenter saw. Compare with the learned-mask rows of Table~\ref {tab:ladder}.\relax }{table.caption.67}{supplementary.pdf}}
\newlabel{tab:posthoc-contact}{{S2.10}{66}{Contact off minus contact on, per axis, paired by patient (post hoc, 12 steps). Columns give the patient-level mean absolute error, the paired difference with its 95\% $t$ CI (df 5) and the patients of 6 sharing its sign. The last four columns split the episodes into the 15 windows where the plane is the skin tangent and the 45 where it is tilted from the skin; they are episode means. No multiplicity adjustment is made and no decision is drawn. $^{\dagger }$Privileged.\relax }{table.caption.68}{supplementary.pdf}}
\newlabel{tab:posthoc-starts}{{S2.11}{66}{Evaluation starts before and after the lift onto the contact plane (post hoc). Offsets are the start translation in the target probe frame. The pre-lift axial offset is the logged offset plus the lift. Positive axial offsets lie deeper than the target face.\relax }{table.caption.69}{supplementary.pdf}}
\newlabel{tab:posthoc-lag}{{S2.12}{67}{Actuation as a lagged position servo (post hoc). Each control step integrates the commanded twist open loop into a target pose and then simulates a short physics interval of a probe welded to that pose. Lag is the distance between the commanded and the actual probe position after each step, pooled over steps, episodes and seeds. Step is the mean commanded translation per step. $^{\dagger }$Privileged.\relax }{table.caption.70}{supplementary.pdf}}
\newlabel{tab:posthoc-horizon}{{S2.13}{67}{The servo base at 12 and 36 steps, contact on (post hoc; the 36-step arms are exploratory). Errors are patient-level mean absolute SE(3)-log components; Out and In are the out-of-plane and in-plane tilts. The base rows pool seeds 0 to 2. The change row is the 36-step minus the 12-step value of the CT-mask base, paired by patient, with its 95\% $t$ CI and $k$/6. Bound rows give the executed twist as a fraction of its bound, averaged over the 12 steps, for the CT-mask base. $^{\dagger }$Privileged.\relax }{table.caption.71}{supplementary.pdf}}
\newlabel{tab:posthoc-lopo}{{S2.14}{68}{Leave-one-patient-out check of the 25 contrasts listed, each printed with 5 of 6 patients sharing its sign (post hoc); other contrasts with 5 of 6 are not checked. Each patient is left out in turn and the mean of the other five is recomputed. Where: where the contrast prints. The sign column says whether all six such means keep the sign of the full mean. Contrasts of the primary results come from the reference evaluation; the others are exploratory.\relax }{table.caption.72}{supplementary.pdf}}
\newlabel{tab:posthoc-s0513}{{S2.15}{68}{Held-out patient s0513 against the other five (post hoc, descriptive). Its start error is 13.12~mm (other five 12.44 to 19.44~mm). Final: patient mean of the final translation error; other five: their range. $S$: match score of the final view against the target; other five: their mean. Static start and pose oracle: 10 episodes of s0513; the other rows pool seeds 0 to 2 (30 episodes). $^{\dagger }$Privileged.\relax }{table.caption.73}{supplementary.pdf}}
\newlabel{tab:posthoc-realism}{{S2.16}{69}{Uncertainty of the distances to real frames of Table~\ref {tab:realism} (post hoc). Point values are those of Table~\ref {tab:realism}. W1 and KID: 95\% percentile intervals of a bootstrap over frames (10,000 resamples; simulated and real frames resampled independently). Resampling biases W1 upward where it is small, so a point value can lie near the lower end of its interval. Null: the classifier two-sample test with the domain labels permuted, 200 permutations per stage. Each permutation is one five-fold run, so its spread is that of a five-fold mean and $p$ is expected to be conservative. $p = (1 + \#\{\text {null} \geq \text {observed}\})/201$, so $1/201$ is the smallest attainable. n/r: no null run. The established-simulator rows of Table~\ref {tab:realism} have no intervals.\relax }{table.caption.74}{supplementary.pdf}}
\newlabel{tab:posthoc-dr-landscape}{{S2.17}{69}{DR landscape over segmenter seeds 0 to 2 (post hoc). Mean per-view Spearman correlation of each term with closeness to the target over the 60 held-out views. Arms: DR off (off), one draw shared by target and samples (shared), independent draws (cross) or a new speckle seed only (cross-seed). Combined: the match score at weights 0.6/0.4. CT-mask terms do not depend on the segmenter seed and print once. Learned-mask terms: the value of each segmenter seed, and their mean with the 95\% $t$ interval over the three seeds (2 df). Seed 0 is the run of \ref {app:dr}. The lower block gives the share of the off arm's combined correlation that the cross arm keeps; the pre-specified rule asks for at least 80\%. $^{\dagger }$Privileged.\relax }{table.caption.75}{supplementary.pdf}}
\newlabel{tab:stats-layers}{{S2.18}{70}{Post hoc statistics layer of Table~\ref {tab:stats-sensitivity} for the learnability, realism, domain-randomization policy and contact contrasts of the primary analysis (6 held-out patients). Columns as in Table~\ref {tab:stats-sensitivity}; Holm within each block. Learnability: difference of the per-patient mean Fisher $z$ of the per-view Spearman correlation. Realism: difference of the per-patient in-sector W1. The four CT-mask servo-base rows of the contact block hold identical episodes by construction and count once; the static start, whose differences are all 0, enters at $p = 1$. Patient $\times $ seed: n/a where a row has no seed factor. $^{\dagger }$Privileged.\relax }{table.caption.76}{supplementary.pdf}}
\newlabel{tab:mixed-model}{{S2.19}{71}{Mixed-model estimates of the final translation error (secondary; never overriding a pre-specified rule; the fits of the primary results are post hoc). Final translation error by arm, with a random intercept for patient and variance components for window and seed within patient. Each model is fitted per question and mask source by restricted maximum likelihood (statsmodels 0.15.0 MixedLM; Nelder-Mead, then Powell in 4 fits). All 16 fits converged. Wald 95\% CIs use the normal quantile, since statsmodels provides no Satterthwaite or Kenward-Roger degrees of freedom. The estimand is conditional on the trained artifacts, with seeds indexing artifacts and the patient as the sampling unit; these intervals do not rest on the patient alone. The model has no arm-by-patient term and one residual variance for all arms of a model, reference rows included. In a contrast of two arms with the same seeds, the patient, window and seed effects cancel. Its interval then rests on that pooled episode-level residual variance and does not carry the between-patient spread of the contrast that the paired $t$ interval carries. In a contrast of an arm with seeds against an arm without seeds or with fewer seeds, the seed variance component enters the interval, which then treats the seeds as sampled. Contrasts between the two mask sources are not modeled, since each model holds one mask source. The planted lateral-bias rows apply the contrasts of the REINFORCE control to the final translation error. The control's rule reads the lateral displacement, which no model here holds, so these rows need not agree with Table~\ref {tab:checks-summary}. Each header gives the fit's variance components as SDs in mm; a component at the boundary was estimated at 0 (the patient component in 14 of 16 fits). $^{\ddagger }$Includes runs that began before their decision rules were fixed. $^{\dagger }$Privileged.\relax }{table.caption.77}{supplementary.pdf}}
\newlabel{fig:stages-twin}{{S3.1}{73}{Supplementary twin of Fig.~\ref {fig:stages}: views of the same held-out patient under the simulators of the renderer slot. Both rows come from patient s0513: the first liver view and the first kidney view of the distance-to-real-frames evaluation, each a randomly perturbed pose near the first screened window. The columns are the authors' physics renderer, the authors' reimplementation of LOTUS, the original LOTUS code with its published default parameters and SIMUS through PyMUST. All four act on the same CT label slice of each view, without a texture stage. Each panel is a sector frame that Table~\ref {tab:realism} scores. The figure is qualitative and exploratory.\relax }{figure.caption.80}{supplementary.pdf}}
\newlabel{supp:perseed}{{S3}{73}{Full table of plugged methods, implementation and compute times}{appendix.supp.3}{supplementary.pdf}}
\newlabel{tab:pluggability-twin}{{S3.1}{74}{Supplementary twin of Table~\ref {tab:pluggability} of the article, with the columns that Table~\ref {tab:pluggability} leaves out: Label, Cost, the paired $t$ $p$, the exact sign-flip $p$, the 90\% $t$ interval of the post hoc TOST, and Score. Exploratory, pre-specified rules. Reference components are marked (authors') or (prior). Values taken from the primary results stay primary. Each slot swaps one component of our reference pipeline. Every run uses the crossed held-out episodes of Table~\ref {tab:ladder} of the article, contact on. Error: final translation error, the mean over seeds of patient-level means. Difference: from the slot's reference component, paired by seed, with its 95\% paired $t$ interval and the patients, of 6, that share its sign. The methods of a family are tested with the two-sided paired $t$-test and Holm's adjustment over all $m$ members. A member without a complete result enters at $p = 1$. The printed Holm $p$ is then an upper bound. $^{\ast }$Holm $p < 0.05$ and at least 5 of 6 patients share the sign. Secondary comparisons are never tested. TOST: post hoc and unadjusted, two one-sided paired $t$-tests at $\pm 1$~mm, the pre-specified margin for the RL change, the label-painted stage and CTA-E; an interval inside $[-1, +1]$~mm shows equivalence within 1~mm. MASK-P (second mask source), IMN-T (pretrained backbone), LPIPS-R (LPIPS reward), CTA-D and CTA-E (CT-anatomy difference and equivalence): later pre-specified families (exploratory, Holm within each, never pooled with the slot families). IMN-T: minus the same network trained from scratch. CTA-E: TOST at $\pm 1$~mm, Holm on the larger $p$, 90\% $t$ interval; there $^{\ast }$ needs no sign count. $^{\dagger }$Privileged: uses simulator state that no physical rig provides. $^{\ddagger }$Fewer seeds than designed, or a learned method below three seeds. Such a row gets no difference. SAM, MedSAM, SAMUS, the look-ahead and SIMUS run seed 0 by design and pair with seed 0 of the reference. BC and DAgger learn from the pose oracle and use BatchNorm in eval mode. Cost: the measurement, unit and device named in each slot header; medians over seeds, except the reward slot's mean per frame pair. Every cost is a benchmark or a timing inside the closed loop. KID and learnability as in the realism and learnability tables of \ref {app:eval}. MedSAM and SAMUS real-frame Dice are not reported, because their pretraining data may include the real test frames.\relax }{table.caption.81}{supplementary.pdf}}
\newlabel{tab:earlier-ctrl}{{S3.2}{76}{Earlier learned-mask controller runs, seeds 0 to 2 (exploratory, no pre-specified rule; run before the learned-mask controller arm was specified). None of these rows enters a decision, and none is read as a separation of two methods. Error: final translation error over the 60 held-out episodes, mean over seeds of patient means. Difference: learner minus the servo base of the same condition, paired by patient, 95\% $t$ CI, with the patients of 6 sharing its sign. Reference rows print their error only. The rerun rows re-evaluate the primary REINFORCE weights in the same evaluation as these learners, so they need not equal the cells of Table~\ref {tab:ladder}.\relax }{table.caption.83}{supplementary.pdf}}
\newlabel{supp:plug-code}{{S3.2}{77}{Code and weights of the plugged methods}{subsection.supp.3.2}{supplementary.pdf}}
\newlabel{tab:compute}{{S3.3}{78}{Hardware and software of USB Gym's runs: every reported result was computed on one Apple M5 Pro laptop with 24~GB of unified memory.\relax }{table.caption.84}{supplementary.pdf}}
\newlabel{supp:compute}{{S3.3}{78}{Compute times}{subsection.supp.3.3}{supplementary.pdf}}
\newlabel{tab:compute-supp}{{S3.4}{79}{Frame, step and training times on the laptop of Table~\ref {tab:compute}. Median [25th, 75th percentile] in ms, batch 1, one process, 5 threads. Physics frame: slice, render, resize and sector warp timed as one block. Closed-loop step: each stage's seed-0 learned-mask policy, 240 steps after 24 warm-up steps; the CPU rows run without the Apple GPU, the MPS rows on it through PyTorch. Texture stage: the stage's generator alone on 200 rendered sector frames after 15 warm-up frames; physics has no texture stage. Training: wall hours per trainer run on the laptop's GPU, median over 3 seeds, with three runs sharing the machine, so upper bounds.\relax }{table.caption.85}{supplementary.pdf}}
\newlabel{tab:learner-settings}{{S3.5}{79}{Settings of the plugged controllers. Every setting was fixed before any run and not tuned on held-out patients: the defaults of Stable-Baselines3 or its RL Zoo scaled to the 57,600-step budget, except SAC and TD3, which take one gradient step per two environment steps at batch 128. Every Stable-Baselines3 learner uses its CnnPolicy (NatureCNN, 512 features) on the stacked frames, a discount of 0.9 and reward normalization. BC and DAgger fit the goal network of the reference trainer to the privileged pose-oracle teacher on 40,000 imitation samples. Residual: a correction bounded at half of $a_{\max }$ added to the servo base; full twist: the whole twist, without the base; 13 moves: no motion or one step per axis and sign.\relax }{table.caption.86}{supplementary.pdf}}
\newlabel{supp:index}{{S4}{80}{Research questions and criteria of the controls}{appendix.supp.4}{supplementary.pdf}}
\newlabel{app:questions}{{S4.1}{80}{Question index}{subsection.supp.4.1}{supplementary.pdf}}
\newlabel{supp:check-rules}{{S4.2}{80}{Criteria of the controls}{subsection.supp.4.2}{supplementary.pdf}}
\newlabel{tab:questions}{{S4.1}{81}{Question index. Unit: the unit of inference, with $n$ in brackets; $n_c$ is the number of cohort cases. Family: the Holm family and its size $m$. Status: ``primary'' marks the pre-specified results of the reference pipeline; ``exploratory, pre-specified rule'' marks a later rule fixed before the data. In the row Estimation-only runs, ``exploratory; estimation only'' marks runs specified after nearly all other results had been seen, with no decision rule. Where no other reason is given, a run that is not reported did not pass the provenance checks. Printed in: the section, appendix, table or figure of the article that prints the result; S2 and S7 are sections of this supplement.\relax }{table.caption.87}{supplementary.pdf}}
\newlabel{tab:checks}{{S4.2}{82}{Controls and exploratory tests (exploratory, pre-specified rules). Each row gives the question that the analysis answers, its criterion fixed before the data and its outcome. Q8 to Q13 and Q2R are questions of the pre-specified exploratory analyses.\relax }{table.caption.89}{supplementary.pdf}}
\newlabel{supp:eval-details}{{S5}{84}{Testbed details and evaluation designs}{appendix.supp.5}{supplementary.pdf}}
\newlabel{app:testbed}{{S5.1}{84}{Testbed details}{subsection.supp.5.1}{supplementary.pdf}}
\newlabel{tab:windows}{{S5.1}{85}{Screened acoustic windows per case. Each window passes the screens of Section~\ref {app:testbed}; liver windows must also show a landmark organ. Kidney targets use flank windows of either side. A case and target enter training or evaluation only with at least 2 windows (kidney counts both sides), so the kidney targets of s0058, s0522 and s0727 are skipped ($^{\dagger }$). Train: 13 cases; held out: 6 cases, used only for evaluation.\relax }{table.caption.93}{supplementary.pdf}}
\newlabel{app:details}{{S5.2}{86}{Task, controller and episode details}{subsection.supp.5.2}{supplementary.pdf}}
\newlabel{app:eval-designs}{{S5.3}{86}{Designs of the Appendix A evaluations}{subsection.supp.5.3}{supplementary.pdf}}
\newlabel{tab:s11-arm-a-secondary}{{S6.1}{89}{Secondary comparisons of the learned-mask controller experiment (secondary; no family, no decision). Learner minus the learned-mask servo base unless the row names another reference; mean over the six held-out patients with the 95\% $t$ CI and the patients of 6 sharing its sign. Units from the metric: mm, deg, the match score $S$, or a fraction of episodes.\relax }{table.caption.106}{supplementary.pdf}}
\newlabel{supp:amend-detail}{{S6}{89}{Additional results of the exploratory experiments}{appendix.supp.6}{supplementary.pdf}}
\newlabel{tab:s11-arm-b-secondary}{{S6.2}{90}{Secondary comparisons of the skin-tangent contact experiment (secondary; no family, no decision): skin-tangent minus target-anchored plane, same rung and seed. Patient-level rows: mean over the six held-out patients with its 95\% $t$ CI; units from the metric. Window rows: the mean episode difference of final translation error (mm) over the windows where the target-anchored plane is tangent to the skin (window tilt below 1$^\circ $) and over the tilted windows (episode level, descriptive).\relax }{table.caption.107}{supplementary.pdf}}
\newlabel{tab:s11-amos-cells}{{S6.3}{91}{The 13 rung and stage cells of the AMOS ordering criterion: final translation error (mm), mean over seeds of case means, on the original six held-out patients, the 30 AMOS CTs and the 20 replication-cohort CTs (descriptive; the three sets are printed side by side and never pooled).\relax }{table.caption.109}{supplementary.pdf}}
\newlabel{tab:s11-amos-cases}{{S6.4}{91}{Per-case descriptors of the 30 AMOS cohort CTs (descriptive). AMOS records no per-case age, sex, institute, study type, vendor or pathology. Split and native slice spacing; axial extent; median HU of the liver and the aorta; fraction of kidney voxels at or above 300~HU; lateral truncation of the kidney slices; screened liver and kidney windows; Dice of the TotalSegmentator v2 labels against the AMOS manual labels (liver; right and left kidney).\relax }{table.caption.110}{supplementary.pdf}}
\newlabel{tab:s11-amos-secondary}{{S6.5}{92}{Secondary comparisons of the AMOS cohort (secondary; no family beyond C3, no decision). Top: REINFORCE final minus after imitation per policy arm, mean with its 90\% $t$ CI. Each arm prints its sign-flip TOST $p$ at $\pm 1$~mm (Monte Carlo, 1,000,000 sign vectors, seed 0); the last row averages the 8 arms. Bottom: the four contrasts without the 9 CTs whose aorta median is at least 300~HU.\relax }{table.caption.111}{supplementary.pdf}}
\newlabel{tab:s11-combination-seeds}{{S6.6}{92}{Per-seed differences of the combination's D and B members (mm; seed $s$ of the combination minus seed $s$ of its reference, for seeds 0, 1 and 2), with the case-by-seed interval: crossed on the 20 cohort CTs and on AMOS, patient by seed on the six (selection-biased; estimation only). AMOS: secondary; estimation only.\relax }{table.caption.112}{supplementary.pdf}}
\newlabel{tab:plug-cohort}{{S6.7}{93}{Plug-cohort rows: each plugged method rerun with its frozen artifacts on the 20 cohort CTs (exploratory; no decision). Mask-source rows are servo bases with the residual off, as on the six patients, and so are the texture rows. Renderer rows are policies trained and evaluated under each renderer, so their six-patient errors differ from Table~\ref {tab:pluggability} of the article. Errors: mean over patients or CTs of the seed-mean final translation error. The last column is a difference of two means, with no interval and no test. $^{\dagger }$Privileged: simulator state that no rig provides. $^{\ddagger }$Fewer seeds than designed: seed 0 only.\relax }{table.caption.113}{supplementary.pdf}}
\newlabel{supp:est}{{S7}{94}{Estimation-only analyses}{appendix.supp.7}{supplementary.pdf}}
\newlabel{supp:est-g2}{{S7.1}{94}{Tissue-anchored speckle in the gap-cause test}{subsection.supp.7.1}{supplementary.pdf}}
\newlabel{supp:est-p9}{{S7.2}{94}{Further pose-free rungs}{subsection.supp.7.2}{supplementary.pdf}}
\newlabel{tab:est-g2-contrasts}{{S7.1}{95}{Tissue-anchored speckle: the look-ahead bound$^{\dagger }$ against the grid-fixed bound$^{\dagger }$, the CT-mask servo base$^{\dagger }$ and the pose oracle$^{\dagger }$, six held-out patients (exploratory; estimation only): 5 contrasts; none adjusted. Every result under the anchored mode is conditional on this renderer with tissue-anchored speckle: no elevational beam width, rigid tissue. $^{\dagger }$Privileged.\relax }{table.caption.114}{supplementary.pdf}}
\newlabel{supp:est-l10}{{S7.3}{96}{Label controls of the per-tissue final policy}{subsection.supp.7.3}{supplementary.pdf}}
\newlabel{supp:est-c30}{{S7.4}{96}{Policies at 36 steps, contact off on the cohort and angiography CTs}{subsection.supp.7.4}{supplementary.pdf}}
\newlabel{tab:est-p9-rung12}{{S7.2}{97}{Pose-free rungs at 12 steps minus the servo base of the same stage, masks and seeds, six held-out patients (exploratory; estimation only): 23 contrasts shown; none adjusted. Under CT masks, the MLP base is read for physics only: its fit for each other stage starts from other random weights, so its 3 rows for those stages are not shown. $^{\dagger }$Privileged.\relax }{table.caption.115}{supplementary.pdf}}
\newlabel{tab:est-p9-rung36}{{S7.3}{98}{Pose-free rungs at 36 steps minus the 36-step servo base, physics frames, six held-out patients (exploratory; estimation only): 7 contrasts; none adjusted. $^{\dagger }$Privileged.\relax }{table.caption.116}{supplementary.pdf}}
\newlabel{tab:est-p9-cohort}{{S7.4}{98}{Pose-free rungs on 20 new CTs minus the servo base of the same stage, masks and seeds (exploratory; estimation only): 12 contrasts; none adjusted. $^{\dagger }$Privileged.\relax }{table.caption.117}{supplementary.pdf}}
\newlabel{tab:est-l10-contrasts}{{S7.5}{98}{Learned-mask final policy of the per-tissue stage: label controls in the closed loop, six held-out patients (secondary; exploratory; estimation only): 5 contrasts; none adjusted.\relax }{table.caption.118}{supplementary.pdf}}
\newlabel{tab:est-c30-c}{{S7.6}{99}{CT-mask policies$^{\dagger }$ evaluated at 36 steps minus the 36-step CT-mask servo base$^{\dagger }$, six held-out patients (descriptive, out of distribution; exploratory; estimation only): 4 contrasts; none adjusted. $^{\dagger }$Privileged.\relax }{table.caption.119}{supplementary.pdf}}
\newlabel{supp:est-r13}{{S7.5}{99}{Planted-deficit control with a larger bias}{subsection.supp.7.5}{supplementary.pdf}}
\newlabel{supp:est-look}{{S7.6}{99}{Look-ahead sampling seeds 1 and 2 on the cohorts}{subsection.supp.7.6}{supplementary.pdf}}
\newlabel{tab:est-c30-d}{{S7.7}{100}{Contact off minus contact on, per rung, 20 new CTs (exploratory; estimation only): 25 contrasts; none adjusted. $^{\dagger }$Privileged.\relax }{table.caption.120}{supplementary.pdf}}
\newlabel{tab:est-c30-e}{{S7.8}{101}{Angiography CTs (a descriptive pool, never combined with the cohort): learned minus CT$^{\dagger }$ masks, SonoSPADE minus physics and the change under REINFORCE per policy arm (exploratory; estimation only): 10 contrasts; none adjusted. $^{\dagger }$Privileged.\relax }{table.caption.121}{supplementary.pdf}}
\newlabel{tab:est-r13-contrasts}{{S7.9}{101}{REINFORCE control with the bias selected on training patients: the planted lateral deficit at iteration 0 ($D_p$) and the recovery statistic $x_p$ per setting, six held-out patients (exploratory; estimation only): 6 contrasts; none adjusted. Every run starts from the CT-mask policy$^{\dagger }$ of the physics stage after imitation. $^{\dagger }$Privileged.\relax }{table.caption.122}{supplementary.pdf}}
\newlabel{tab:est-look-contrasts}{{S7.10}{101}{Look-ahead sampling seeds 0 to 2 averaged: the look-ahead bound$^{\dagger }$ minus the mean of the CT-mask servo base$^{\dagger }$ over its calibration seeds, on both cohorts (exploratory; estimation only): 2 contrasts; none adjusted. $^{\mathrm {MC}}$Monte Carlo sign-flip $p$ (1,000,000 sign vectors, seed 0). Both rows are conditional on this renderer: grid-fixed speckle, no elevational beam width, rigid tissue. $^{\dagger }$Privileged.\relax }{table.caption.123}{supplementary.pdf}}
\makeatother
